# Supplementary material for: DeltaCam: Differential Intrinsic Camera Modeling for Video Generation
Source: arXiv:2605.25266 source file (2026-05-24)
Supplement: Supplementary file 1 [file supp_algo.tex]

% \begin{figure*}[t]
%     \centering
%     \begin{minipage}[t]{0.47\textwidth}
%       \begin{lstlisting}[style=pseudocode]
%   def style_extract(X: (B, T, 3, H, W), concepts: List[str]):

%       # per-frame backbone (frozen c-RADIO v4 ViT-H)
%       summary, patches = cRADIO(X)           # (B,T,1280), (B,T,N,1280)
%       pooled = GaussianPool(patches, $\sigma$=0.3)  # uniform + radial + centre
%       H = Linear([summary; pooled])          # (B, T, 1280)

%       # shared temporal encoder
%       H = TransformerEncoder(H + SinPE,      # 4 layers, 8 heads,
%                              d=1280)         # feedforward = 4d

%       # content branch  ->  scene-identity vector
%       z_c = MLP(CrossAttn(q_learned, H))    # (B, 256),  depths 1280->2560->256

%       # style branch  ->  per-frame embeddings
%       Z_s = TransformerEncoder(H + SinPE,   # 4 layers, 8 heads
%                                d=1280)
%       Z_s = MLP(Z_s)                        # (B, T, 256),  1280->256

%       # per-concept trajectory heads
%       trajs = {}
%       for c in concepts:
%           trajs[c] = Linear(GELU(Linear(Z_s,  # 256 -> 128
%                                  128)), 1)    # 128 -> 1,  z-scored
%       return z_c, Z_s, trajs
%       \end{lstlisting}
%       \captionof{lstlisting}{Style extraction forward pass (one model per effect).}
%       \label{alg:style}
%     \end{minipage}    
%     \hfill
%     \begin{minipage}[t]{0.47\textwidth}
%       \begin{lstlisting}[style=pseudocode]
%   def recam_inference(X_src: (B,T,3,H,W), $\tau$: Dict[effect, (T,)],
%                       prompt: str, N: int = 50):

%       # --- proxy stream extraction (frozen) ---
%       D = DepthEstimator(X_src)           # (B, T, 1, H, W)
%       F = OpticalFlow(X_src)              # (B, T, 2, H, W)
%       P = PerspectiveField(X_src)         # (B, T, 4, H, W)

%       # --- VAE encoding ---
%       z_src   = VAE.encode(X_src)         # (B, 16, T', H', W')
%       z_depth = VAE.encode(D)             # (B, 16, T', H', W')
%       z_flow  = VAE.encode_multichan(F)   # (B, 32, T', H', W')
%       z_pf    = VAE.encode_multichan(P)   # (B, 64, T', H', W')

%       # --- camera control module (CCM) ---
%       x2d = [z_depth, z_flow, z_pf, z_src]
%       x1d = build_x1d($\tau$)                   # (B, 6, T', 8)
%       x1d_norm = [x1d_enc[j](x1d[:,j]) for j in effects]
%       acc = $\sum_{k,j}$ FiLM(InputProj(x2d[k]), x1d_norm[j])
%       for stage in [0, 1, 2]:
%           acc = CausalTemporalSelfAttn(StageProj(acc))
%       cam_emb1 = [OutProj[b](acc) for b in DiT.blocks]

%       # --- diffusion denoising loop ---
%       z = randn_like(z_src)
%       for t in FlowMatchScheduler.timesteps(N):
%           z_in = concat([z, z_src], dim=T)
%           x = PatchEmbed(z_in);  e = patchify1(cam_emb1)
%           for b, block in enumerate(DiT.blocks):
%               $\tilde{x}$ = AdaLN(x, t)
%               x1 = SA(    $\tilde{x}$ + CamEnc(e_scalar))
%               x2 = SA_eff($\tilde{x}$ + e[b])
%               x = x + $g_\text{msa}$ * 0.5*(P1(x1) + P2(x2))
%               x = x + CrossAttn(x, context) + $g_\text{mlp}$*FFN(AdaLN(x,t))
%           z = scheduler.step(Head(x), t, z)

%       return VAE.decode(z)                 # (B, T, 3, H, W)
%       \end{lstlisting}
%       \captionof{lstlisting}{Camera-conditioned VDM inference forward pass.}
%       \label{alg:inference}
%     \end{minipage}
%   \end{figure*}

\begin{figure*}[t]
    \centering
    \begin{minipage}[t]{0.47\textwidth}
      \begin{lstlisting}[style=pseudocode]
  def vdm_inference(X_src: (B,T,3,H,W), $\tau$: Dict[effect, (T,)],
                    prompt: str, N: int = 50):
  
      # --- proxy stream extraction (frozen) ---
      D = DepthEstimator(X_src)           # (B, T, 1, H, W)
      F = OpticalFlow(X_src)              # (B, T, 2, H, W)
      P = PerspectiveField(X_src)         # (B, T, 4, H, W)
  
      # --- VAE encoding ---
      z_src   = VAE.encode(X_src)         # (B, 16, T', H', W')
      z_depth = VAE.encode(D)             # (B, 16, T', H', W')
      z_flow  = VAE.encode_multichan(F)   # (B, 32, T', H', W')
      z_pf    = VAE.encode_multichan(P)   # (B, 64, T', H', W')

      # --- camera control module (CCM) ---
      x2d = [z_depth, z_flow, z_pf, z_src]
      x1d = build_x1d($\tau$)                   # (B, 6, T', 8)
      x1d_norm = [x1d_enc[j](x1d[:,j]) for j in effects]
      acc = $\sum_{k,j}$ FiLM(InputProj(x2d[k]), x1d_norm[j])
      for stage in [0, 1, 2]:
          acc = CausalTemporalSelfAttn(StageProj(acc))
      cam_emb1 = [OutProj[b](acc) for b in DiT.blocks]
  
      # --- diffusion denoising loop ---
      z = randn_like(z_src)
      for t in FlowMatchScheduler.timesteps(N):
          z_in = concat([z, z_src], dim=T)
          x = PatchEmbed(z_in);  e = patchify1(cam_emb1)
          for b, block in enumerate(DiT.blocks):
              $\tilde{x}$ = AdaLN(x, t)
              x1 = SA(    $\tilde{x}$ + CamEnc(e_scalar))
              x2 = SA_eff($\tilde{x}$ + e[b])
              x = x + $g_\text{msa}$ * 0.5*(P1(x1) + P2(x2))
              x = x + CrossAttn(x, context) + $g_\text{mlp}$*FFN(AdaLN(x,t))
          z = scheduler.step(Head(x), t, z)
  
      return VAE.decode(z)                 # (B, T, 3, H, W)
      \end{lstlisting}
      \captionof{lstlisting}{Camera-conditioned VDM inference forward pass.}
      \label{alg:inference}
    \end{minipage}
    \hfill
    \begin{minipage}[t]{0.52\textwidth}
      \begin{lstlisting}[style=pseudocode]
  def style_extract(X: (B, T, 3, H, W), concepts: List[str]):

      # per-frame backbone (frozen c-RADIO v4 ViT-H)
      summary, patches = cRADIO(X)           # (B,T,1280), (B,T,N,1280)
      pooled = GaussianPool(patches, $\sigma$=0.3)  # uniform + radial + centre
      H = Linear([summary; pooled])          # (B, T, 1280)
  
      # shared temporal encoder
      H = TransformerEncoder(H + SinPE,      # 4 layers, 8 heads,
                             d=1280)         # feedforward = 4d

      # content branch  ->  scene-identity vector
      z_c = MLP(CrossAttn(q_learned, H))    # (B, 256),
                                            #  depths 1280->2560->256

      # style branch  ->  per-frame embeddings
      Z_s = TransformerEncoder(H + SinPE,   # 4 layers, 8 heads
                               d=1280)
      Z_s = MLP(Z_s)                        # (B, T, 256),  1280->256
  
      # per-concept trajectory heads
      trajs = {}
      for c in concepts:
          trajs[c] = Linear(GELU(Linear(Z_s,  # 256 -> 128
                                 128)), 1)    # 128 -> 1,  z-scored
      return z_c, Z_s, trajs
      \end{lstlisting}
      \captionof{lstlisting}{Style extraction forward pass (one model per pass).}
      \label{alg:style}
    \end{minipage}
  \end{figure*}

  


% \begin{figure}[t]
%   \begin{lstlisting}[style=pseudocode,
%     caption={Style extraction forward pass (one model per effect).},
%     label={alg:forward}]
%   def style_extract(X: (B, T, 3, H, W), concepts: List[str]):

%       # per-frame backbone (frozen c-RADIO v4 ViT-H)
%       summary, patches = cRADIO(X)           # (B,T,1280), (B,T,N,1280)
%       pooled = GaussianPool(patches, $\sigma$=0.3)  # uniform + radial + centre
%       H = Linear([summary; pooled])          # (B, T, 1280)

%       # shared temporal encoder
%       H = TransformerEncoder(H + SinPE,      # 4 layers, 8 heads,
%                              d=1280)         # feedforward = 4d

%       # content branch  ->  scene-identity vector
%       z_c = MLP(CrossAttn(q_learned, H))    # (B, 256),  depths 1280->2560->256

%       # style branch  ->  per-frame embeddings
%       Z_s = TransformerEncoder(H + SinPE,   # 4 layers, 8 heads
%                                d=1280)
%       Z_s = MLP(Z_s)                        # (B, T, 256),  1280->256

%       # per-concept trajectory heads
%       trajs = {}
%       for c in concepts:
%           trajs[c] = Linear(GELU(Linear(Z_s,  # 256 -> 128
%                                  128)), 1)    # 128 -> 1,  z-scored
%       return z_c, Z_s, trajs
%   \end{lstlisting}
%   \end{figure}
