# Supplementary material for: DeltaCam: Differential Intrinsic Camera Modeling for Video Generation
Source: arXiv:2605.25266 source file (2026-05-24)
Supplement: Supplementary file 2 [file supplement.tex]

\input{content/supplement/0-how-to-use}
