# Supplementary material for: DeltaCam: Differential Intrinsic Camera Modeling for Video Generation
Source: arXiv:2605.25266 source file (2026-05-24)
Supplement: Supplementary file 3 [file 0-how-to-use.tex]

% Uncomment next line to make a one-column supplement
\onecolumn

\section{Implementation Details}
\subsection{Extended Training Mechanics and Gradient Routing}
\label{sec:supp_training}

Our three-stage training curriculum is designed to progressively inject explicit camera control into a pre-trained Video Diffusion Model (VDM) while strictly preventing catastrophic forgetting of the base model's dynamic priors. 

\paragraph{Stage 1: Base Camera Model Pre-training.} 
The objective of the first stage is to align the spatial layers of the VDM with our synthetic $\Delta$-parameterized control space. We inject the dual conditioning streams---camera pose $\mathbf{P}$ (extrinsics) and relative photographic trajectories $\Delta\boldsymbol{\theta}_t$ (intrinsics)---directly into the inflated self-attention blocks of the VDM. To ensure the conditioning correctly modulates the visual features, the vectors are concatenated with the video latent $\mathbf{z}_t$ and passed through independent self-attention heads prior to final feature fusion. Because video generation is highly sensitive to temporal jitter, we strictly freeze all temporal transformer layers within both the VDM and the camera encoder. Consequently, gradients only update the Camera Conditioning Module (CCM) and the spatial attention weights, ensuring the backbone's temporal consistency remains intact.

\paragraph{Stage 2: Style Transfer Adaptation.} 
Once the spatial layers accurately interpret the synthetic $\Delta\boldsymbol{\theta}_t$ controls, we decouple the generative backbone from the style extraction process. We freeze the entirety of the VDM and the core CCM. Training is restricted exclusively to the lightweight style extractor adaptor (style transfer ViT remains frozen) introduced in the main text. By isolating gradients to this specific module, the network learns to regress the extracted style embedding $\mathbf{z}_s$ into the exact $\Delta$-parameter space expected by the frozen CCM, preventing any degradation of the base generation quality during reference-driven tasks.

\paragraph{Stage 3: Real-World Shot Matching.} 
The final stage grounds the synthetic priors to absolute, real-world camera states. We maintain the frozen state of the VDM, the temporal layers, and the core CCM. We fine-tune only the lightweight EXIF metadata tokenizer $\Phi_{\text{meta}}$ (implemented as a two-layer MLP with SiLU activations). By restricting the gradient updates solely to this adaptor, the MLP learns a continuous mapping from the normalized absolute metadata sequence $\boldsymbol{\xi}_t$ into our pre-trained synthetic control manifold. This isolated fine-tuning acts as a domain bridge, enabling precise, camera-specific shot emulation from real-world EXIF data without requiring expensive retraining of the diffusion backbone.


% \section{Tables}
% \input{content/tables/dataset_cfe}
\subsection{Neural Network Details}
\label{sec:model}
    Listing~\ref{alg:inference} details our camera controlled video generation model's forward pass.
  \paragraph{\textbf{VDM Architecture.}}
  The camera conditioning module (CCM) is implemented as a stack of 3 group-cascaded FilM encoder followed by two causal temporal self-attention blocks (8 heads, \texttt{channels}$=[256,256,256]$), repeated 3 times.
  2D proxy streams (depth, optical flow, perspective field, source video) are projected
  via per-stream input convolutions with channel widths $\mathbf{c}_{2D}=[16,32,64,16]$.
  The 1D trajectory vector is zero-padded to a fixed width $c_{1D}=8$, then modulated into
  each stage via a FiLM MLP: a two-layer network Linear$(8,256)$\,+\,SiLU\,+\,Linear$(256,2c_{\mathrm{out}})$
  with the output layer zero-initialized.
  Each stage outputs $c_{\mathrm{cam}}=16$ channels projected linearly into every DiT block.

  \paragraph{Effect attention injection.}
  Each DiT block is augmented with a dual-stream self-attention mechanism.
  The CCM produces a per-block feature map of $c_\text{cam}=16$ channels,
  which is patchified into token space by a learned 3-D convolutional patch embedding, same kernel and stride as the main patch embedding).
  Inside each block, two parallel self-attention streams are computed on the
  layer normalized input from previous block ($\tilde{z_t}$):
  \begin{enumerate}[leftmargin=1.5em, itemsep=0pt]
    \item \textbf{Content stream.} Original self-attention applied to video tokens augmented
          with a per-frame scalar camera embedding (Linear $12\!\to\!d_\text{DiT}$, zero-initialized).
    \item \textbf{Effect stream.} A copy of the content stream self-attention applied to video tokens augmented with the patchified-CCM tokens.
  \end{enumerate}
  Their outputs are averaged with equal weight and gated by the AdaLN gate:
  \begin{equation}
    z_t \leftarrow z_t + g_\text{msa}\cdot\tfrac{1}{2}
      \bigl(P_1(\mathrm{SA}(\tilde{z_t}+e_\text{cam})) + P_2(\mathrm{SA}_\text{eff}(\tilde{z_t}+e_\text{CCM}))\bigr),
  \end{equation}
  where $\tilde{z_t}$ is the AdaLN-modulated input, $g_\text{msa}$ is the AdaLN gate,
  $e_\text{cam}$ is the per-frame scalar embedding, $e_\text{CCM}$ are the patchified CCM tokens,
  and $P_1, P_2$ are linear projectors initialized to the identity.
  During training only the effect self-attention, effect patch embedding layer,
  and $P_2$ are trainable; the rest of the DiT backbone remains frozen.

  \paragraph{Trajectory normalization.}
  Per-effect 1D trajectories are linearly mapped to $[0,1]$ before encoding:
  Bokeh ($K\!\in\![0,25]$, focus$\,\in[0,1]$, 2-dim),
  Exposure ($\mathrm{EV}\!\in\![-3,3]$, 1-dim),
  Zooming (focal length $f\!\in\![25,100]$\,mm, 1-dim),
  Temperature ($T\!\in\![3000,9000]$\,K, 1-dim), 
  Fisheye ($\xi\!\in\![0,1.8]$, lensmode, zoom, 3-dim) and
  Shutter ($FPS\!\in\![5, 50]$, 1-dim).

  \paragraph{Training objective.}
  We minimize the flow-matching denoising loss
  \begin{equation}
    \mathcal{L} = \mathbb{E}_{t,\mathbf{x},\boldsymbol{\epsilon}}
      \bigl[w(t)\,\|\hat{\mathbf{v}}_\theta(\mathbf{x}_t) - \mathbf{v}_t\|^2\bigr],
  \end{equation}
  where $w(t)$ is the SNR-based training weight from the WAN flow-matching scheduler and
  $\mathbf{v}_t$ is the velocity target. No auxiliary losses are used.

  \paragraph{Optimization.}
  We use AdamW ($\beta_1{=}0.9$, $\beta_2{=}0.999$, $\varepsilon{=}10^{-8}$,
  weight decay$\,{=}0.01$) with learning rate $10^{-5}$, gradient clipping at norm 1.0,
  batch size 1, and no gradient accumulation.
  The DiT backbone is kept frozen throughout; only the CCM parameters and  are trained.
  Training runs for 3\,750 steps on a single NVIDIA A100 GPU
  (approx.\ \textbf{288} GPU-hours). Training loss trajectory is shown in \cref{fig:loss}.
  \input{content/figures/loss}

  \paragraph{Camera-matching fine-tuning.}
  For fine-tuning on real paired data with EXIF metadata, we additionally freeze the
  causal temporal effect and pose attention blocks and the pose projection layers, and train only the per-effect 1D metadata encoder adaptor $\Phi_{meta}$, input projections, and output projection heads.
  The metadata encoder uses learning rate $5\!\times\!10^{-5}$ and all other trained parameters
  use $10^{-5}$; gradient accumulation is set to 4 steps (effective batch size 4).
  EXIF fields (e.g., \textit{Aperture}, \textit{FocalLength}, \textit{ISO}) are read from
  JSON sidecars, cast to float, and fed directly into the 1d slider control slot for the target effect;
  missing fields receive fill value 0.

\input{content/figures/supp_algo}
\paragraph{\textbf{Style Extraction Module Architecture.}}
  Listing~\ref{alg:style} details the forward pass.
  The backbone (c-RADIO v4 ViT-H, frozen) outputs a summary token and patch tokens per
  frame; patch tokens are Gaussian-pooled ($\sigma{=}0.3$) into three spatial maps
  (uniform, radial, centre-weighted) and projected with the summary to $d{=}1280$.
  A four-layer sinusoidal-PE transformer ($8$ heads, feedforward $4d$) encodes the
  $T{=}16$ frame sequence.
  The content encoder pools this into a single vector via cross-attention and a
  three-layer MLP ($1280{\to}2560{\to}256$).
  The style encoder runs a second four-layer transformer followed by a two-layer MLP
  ($1280{\to}256$) to produce per-frame embeddings.
  Each photographic concept has an independent two-layer head
  ($256{\to}128{\to}1$) predicting a z-scored scalar per frame.
  Total trainable parameters: $562$M.

  \paragraph{Training.}
  We train one model per photographic effect on RealCam-Vid using AdamW
  ($\beta_1{=}0.9$, $\beta_2{=}0.999$, weight decay $5{\times}10^{-5}$)
  at learning rate $3{\times}10^{-6}$ with a one-epoch linear warm-up and cosine
  decay over $100$ epochs.
  Batches contain $5$ videos each expanded to $6$ trajectory augmentations
  ($30$ effective samples), processed at $336{\times}336$ with $T{=}16$ frames.
  Gradients are clipped to norm $10$.

  \paragraph{Loss weights.}
  The trajectory NCC loss uses $\lambda_\tau{=}2.0$; content and style InfoNCE use
  $\lambda_c{=}0.1$ and $\lambda_s{=}0.3$ with temperature $\tau{=}0.07$; the MI
  penalty uses $\lambda_\text{MI}{=}0.05$.
  For most effects a flat-trajectory variance penalty ($\lambda_\text{flat}{=}0.1$),
  temporal smoothness ($\lambda_\text{smooth}{=}0.005$), and z-score range penalty
  ($\lambda_\text{range}{=}0.05$) are also applied;
  these are set to zero for the bokeh and motion-blur effects,
  where mutually exclusive rendering modes would cause the flat penalty to compete
  with NCC.


\subsection{Architectural Choices} 
% \cref{fig:ccm_evolution}
\input{content/figures/archi_evolution}

\label{sec:supp_arch_choices}

This section documents key architectural decisions across DeltaCam and the alternatives we considered.

\paragraph{CCM evolution.}
The CCM design (\cref{fig:ccm_evolution}) emerged from four iterations. Our initial design (V1) used StyleGAN2-style weight modulation (StyleMod)~\cite{karras2020analyzing} with per-effect convolutional proxy encoders, which produced unstable training and rapid collapse to near-zero modulations. We attribute this to the multiplicative weight-update form producing rapidly varying per-layer gradients in the small-$\Delta\boldsymbol{\theta}_t$ regime dominant in our training. In V2, we substitute StyleMod with AdaIN~\cite{huang2017arbitrary} on the optical group, which stabilizes that branch but left the sensory and ISP branches unstable. In V3,  we replaced all modulation with FiLM~\cite{Perez2017FiLMVR}, whose additive scale-and-shift form keeps gradients bounded and, combined with zero-initialized heads, allows the model to start from an identity mapping and depart gradually. In the final version, we replaced the convolutional proxy encoders with the same frozen 3D VAE used by the VDM, thus ensuring proxy features live in the VDM's native latent space and adding no trainable parameters, and split intrinsics into three physically grouped FiLM cascades (optical $\{f, f/\#, \xi\}$, sensory $\{s, \text{EV}\}$, ISP $\{K\}$) so each group's weights update only when its supervising effect is active.

\paragraph{Why every spatial proxy is routed to every effect.}
A natural alternative is to wire individual proxies to specific effects (e.g., depth only for Bokeh, RGB only for color temperature). We instead route all proxies to all effects. Our FiLM-magnitude visualization (\cref{fig:ablations}) shows every effect draws non-trivial signal from multiple proxies---photometric effects activate source RGB most strongly, geometric effects favor depth and perspective field, but no effect uses only a single proxy. Selective wiring would forfeit this redundancy, which we observe helps in challenging scenarios where one proxy estimator becomes unreliable (e.g., monocular depth on transparent surfaces). The remaining cross-group cross-talk is benign: when an effect is inactive ($\Delta\theta = 0$), FiLM reduces to identity, so inactive groups contribute nothing without explicit gating.

\paragraph{Frame embedder choice: C-RADIO ViT-H.}
The style extractor (\cref{sec:style_understanding}) requires a frozen frame embedder that captures both semantic content and fine spatial structure. The former for content/style separation, the latter for resolving effects like bokeh and lens distortion that manifest as spatial cues. We use C-RADIO ViT-H~\cite{ranzinger2026cradiov4techreport}, an agglomerative foundation model trained to align features across DINOv2\cite{oquab2023dinov2}, CLIP \cite{radford2021learning}, and SAM \cite{kirillov2023segment}. This pretraining gives a single backbone access to DINOv2's spatial structure, CLIP's semantic alignment, and SAM's segmentation priors.

\paragraph{Loss design.}
We use InfoNCE on both content and style branches as the primary disentanglement objective, plus a squared-cosine mutual information term. The MI term guards against shortcut learning in the semi-supervised regime: with limited paired training data, the contrastive objective alone admits solutions where content and style embeddings remain partially correlated. The MI loss explicitly penalizes residual correlation, providing an additional disentanglement signal. Loss weights $\lambda_\tau, \lambda_c, \lambda_s, \lambda_{\text{MI}}$ were selected via grid search; full values were in reported in previous subsection.


\section{Dataset details}

\subsection{Spatial Proxy Implementation} 
We implement the spatial proxies using
  Depth Anything V2~\cite{yang2024depthanythingunleashingpower} for monocular depth,
  RAFT~\cite{teed2020raftrecurrentallpairsfield} for optical flow,
  and perspective fields from~\cite{jin2023perspective}.
  Depth maps are estimated per-frame and min-max normalized to $[0,1]$.
  Optical flow is computed between consecutive frames and normalized globally.
  Perspective fields provide a 4-channel map of gravity direction and
  surface latitude, encoding scene upright orientation.
  These three spatial proxies, together with the source video latent,
  form the four 2D conditioning streams fed to the CCM
  ($\mathbf{c}_{2D} = [16, 32, 64, 16]$ latent channels respectively).
  All proxy models are frozen throughout training.

\subsection{Synthetic Camera Video  
Pipeline}

All effects are applied to source video clips on the GPU.
  Trajectories are generated as smooth spline curves with random
  start/end values and 1–3 interior anchor points, clamped to
  per-effect physical ranges.
  Below we describe each effect pipeline.

  \paragraph{Bokeh (depth-of-field blur).}
  Per-frame disparity maps are estimated by Depth Anything V2 (frozen)
  and min-max normalized to $[0,1]$.
  A scatter-based classical renderer~\cite{peng2022bokehme}
  computes depth-dependent defocus using:
  \begin{equation}
    \delta(p) = K \cdot \frac{d(p) - d_\text{focus}}{10},
  \end{equation}
  where $K\in[0,25]$ is the blur strength and $d_\text{focus}\in[0,1]$
  is the normalized focus plane depth.
  Images are linearized ($\gamma=2.2$) before scattering and
  de-linearized after.
  
  % The 2D proxy encodes three channels:
  % normalized blur magnitude $|\delta|$, focus mask $1-|d-d_\text{focus}|$,
  % and raw disparity.

  
  \paragraph{Exposure control.} Rather than modeling ISO sensitivity as a monolithic noise process, we decompose its
  photographic effects into two orthogonal factors already present in our pipeline:
  exposure gain (EV, which captures the brightness amplification that higher ISO provides)
  and shutter speed (which controls motion blur duration, as slower shutters accompany
  high-ISO low-light capture). This factorization avoids entangling sensor noise statistics
  with photometric and geometric effects, enabling cleaner independent control over each factor.
  Exposure is parameterized in EV stops, $\Delta\mathrm{EV}\in[-3,3]$.
  Each frame is first linearized via inverse gamma ($\gamma=2.2$),
  then scaled by the linear gain $g=2^{\Delta\mathrm{EV}}$,
  clipped to $[0,1]$ to simulate sensor saturation,
  and re-gamma-encoded:
  \begin{equation}
    I_\text{out} = \bigl(\min(I_\text{lin}\cdot 2^{\Delta\mathrm{EV}},\,1)\bigr)^{1/\gamma}.
  \end{equation}
  The 1D trajectory is a single scalar per frame.
  
  \paragraph{Cinematic blur (shutter / motion blur).}
  RAFT optical flow~\cite{teed2020raftrecurrentallpairsfield} is computed between consecutive
  frames and scaled by a per-frame shutter scalar
  $s = \mathrm{clip}((\text{base\_fps}\,/\,\text{target\_fps}),\;0.5,\;4.0)$.
  Both the scalar trajectory and the mean flow direction are independently
  smoothed with a length-5 temporal box filter before use, suppressing
  intensity-pumping and background-vibration artifacts.
  Rather than mixing blur modes per frame, the pipeline commits to a single
  rendering mode for the entire clip based on the clip-level mean standard deviation
  of per-pixel flow magnitudes: if $\bar{\sigma}_\text{flow} > 5.0$\,px the clip is
  treated as exhibiting complex \emph{object motion} and blur is applied via
  24 pixel-window accumulation along per-pixel flow vectors;
  otherwise a global \emph{camera motion} model is used, convolving each frame
  with a direction-aligned Gaussian kernel ($33{\times}33$, thickness 1.5\,px)
  derived from the smoothed mean flow.
  The 1D trajectory encodes the shutter speed scalar.

  \paragraph{Color temperature (warmth).}
  White balance is shifted by multiplying each frame (in $[0,1]$) by a
  per-channel RGB gain derived from a Kelvin-to-RGB analytic curve
  (Tanner Helland's algorithm, $T\in[3000,9000]$\,K):
  \begin{equation}
    I_\text{out}^c = \mathrm{clip}\!\left(I^c \cdot g_c(T),\,0,1\right), \quad c\in\{R,G,B\}.
  \end{equation}
  Warm values ($T\approx3000$\,K) boost red/green and suppress blue;
  cool values ($T\approx9000$\,K) do the reverse.

  \paragraph{Fisheye distortion.}
  The Unified Sphere Model (USM)~\cite{mei2007single} is used to simulate fisheye optics.
  Given $\xi\in[0.2,\,1.4]$ (pure barrel; $\xi>0$), image coordinates are scaled by
  $z=0.7/(1+\xi)$ to prevent black borders.
  The inverse USM formula maps each output pixel to a 3-D ray:
  \begin{align}
    \alpha &= \frac{\xi + \sqrt{1 + (1-\xi^2)(u^2+v^2)}}{1 + u^2 + v^2}, \\
    (d_x, d_y, d_z) &= (\alpha u,\; \alpha v,\; \alpha - \xi),
  \end{align}
  which is re-projected via $(d_x/d_z,\,d_y/d_z)$ and bounding-box-normalized to
  $[-1,1]$ before bicubic \texttt{grid\_sample}.
  % The 2D proxy is a 3-channel pixel displacement field $[\Delta x,\,\Delta y,\,\|\Delta\|]$
  % (difference between distorted and undistorted sampling coordinates),
  % together with a broadcast 1D style map $[\xi,\,z,\,\text{lensmode}]$.
  A radial vignette ($\text{strength}=0.6$) is applied after warping. A radial vignette ($\text{strength}=0.6$) is applied after warping.
  The USM model naturally extends to other lens distortions —
  pincushion distortion, for instance, is obtained by negating $\xi$
  ($\xi < 0$) without any architectural change;
  we leave exploration of these modes to future work.

  \paragraph{Focal zoom control (supersampling).}
  Zoom is simulated by an affine crop-and-resize using normalized
  sampling coordinates.
  The scale factor $s=f_0/f$ (with base focal length $f_0=25$\,mm,
  $f\in[25,100]$\,mm) shrinks the sampling region proportionally to
  the zoom level.
  A key design choice is \emph{relative-coordinate supersampling}: the
  affine grid is defined in normalized coordinates $[-1,1]$, making it
  resolution-agnostic.
  Source frames are held at the full native resolution ($>$480p),
  so the center crop at zoom level $f$ spans
  $\lfloor H/s\rfloor\times\lfloor W/s\rfloor$ pixels in the source —
  significantly more than the output grid requires.
  Bicubic grid sampling then compresses these into the output
  resolution, giving anti-aliased zoom with no pre-downsampling step.
  At maximum zoom ($f=100$\,mm, $s=0.25$) the sampled region is
  120$\times$208 px from the 480$\times$832 source, yielding a 4$\times$
  effective supersampling factor at the output.
  % The 2D proxy is a binary center-crop mask scaled by $s$.

  \input{content/figures/dataset_preview}
\subsection{Real Video Datasets} 
We evaluate on two complementary sources, illustrated in \cref{fig:dataset_composition}.

  \textbf{RealCam-Vid}~\cite{li2025realcam} aggregates ${\sim}100$K real-world video clips
  from three public collections — RealEstate10K,
  DL3DV-10K, and MiraData,
  unified under a common metric-scale camera annotation.
  RealEstate10K and DL3DV provide static indoor and outdoor scenes with
  high-quality SLAM/COLMAP camera tracks, while MiraData contributes
  dynamic scenes with concurrent object motion and camera movement.
  Camera poses across all three sources are re-estimated with
  MonST3R~\cite{zhang2025monst3r}, which explicitly handles moving
  foreground objects, and aligned to a shared metric scale via a
  per-clip scale factor.
  This gives a diverse split of static and dynamic content with
  consistent, physically meaningful camera trajectories.

  \textbf{MultiCamVideo}~\cite{bai2025recammaster} is a large-scale
  synthetic dataset rendered in Unreal Engine~5, comprising 13,600
  dynamic scenes each captured by 10 time-synchronized cameras,
  yielding 136K video clips at $1280{\times}1280$ resolution (81 frames,
  15 fps).
  Each scene pairs a photorealistic 3D environment with animated human
  characters and randomized camera trajectories spanning pan/tilt,
  translation, arc, and freeform motion.
  Four camera configurations are provided — focal lengths of
  \{18, 24, 35, 50\}\,mm and apertures of \{2.4, 5.0, 10.0\} —
  enabling controlled study of lens-induced photometric effects such as
  depth-of-field blur alongside geometric camera motion.


\subsection{Real EXIF-Image Camera Datasets} 

\paragraph{Camera Matching Dataset Adaptation.}
  Real-camera effect datasets such as \emph{RealBokeh} (aperture-sweep image pairs),
  \emph{Zoom} (focal-length sweep scenes), and \emph{NeuralCam} (ISO-sweep scenes)
  consist of still image pairs $(I_\text{src}, I_\text{gt})$ rather than continuous videos,
  and carry discrete per-image EXIF metadata instead of smooth per-frame trajectories.
  As illustrated in ~\cref{fig:cam_adapt}, adapting these to our video diffusion
  backbone requires bridging two structural gaps.
  First, each still image is inflated into a static pseudo-video by replicating it
  across all $T{=}81$ frames, producing a latent of shape $[16, T', H', W']$
  identical in format to a real video clip, with no temporal variation.
  A single depth map is estimated from the source image (Depth Anything V2, frozen)
  and replicated likewise.
  Second, since no camera motion is present, all extrinsic conditioning
  (optical flow, perspective field) is zeroed out; only the 1D EXIF vector
  occupies the slider control slot for the target effect.
  EXIF fields (\emph{e.g.}, Aperture, FocalLength, ISO) are read from the image metadata using \texttt{rawpy}.

  % \paragraph{Training protocol.}
  % All latents are pre-computed once (VAE-encoded source, target, and depth)
  % and cached as \texttt{.pth} files, so training iterates over latent tensors
  % directly without re-running the VAE.
  % The DiT backbone, causal temporal attention blocks, and stage projections remain
  % frozen; only the per-effect 1D encoder, FiLM layers, input projections, and
  % output projection heads are updated (see Sec.~\ref{sec:impl}).
  % Unlike the pre-training phase where trajectories are dense smooth splines sampled
  % continuously from physical ranges, the fine-tuning supervision signal comes
  % from discrete $(I_\text{src}, I_\text{gt})$ pairs at fixed EXIF settings,
  % \emph{e.g.}, a single jump from $f/22$ to $f/2.8$ for bokeh,
  % or from $24$\,mm to $200$\,mm for zoom.
  % This discrete, image-level supervision teaches the x1d encoder to align
  % real EXIF units with the physical parameter space learned during pre-training,
  % without disrupting the temporal dynamics acquired from video data.

% \cref{fig:cam_adapt}
\input{content/figures/cam_data_adaptation}

\section{Extended Ablations}

\input{content/figures/fidelity}
\subsection*{Effect Fidelity}

  We measure how reliably the model follows the requested effect intensity.
  For each effect, we sweep its control parameter across ten evenly-spaced levels
  and generate a video at each level using a fixed scene.
  We extract a proxy signal from the output frames:
  mean luminance for Exposure, red-to-blue channel ratio for Temperature,
  edge density for Zooming, and inverse variance-of-Laplacian for Bokeh.
  We compute Pearson $r$ between the requested intensity trajectory and the measured signal
  and plot the correlation curves in \cref{fig:fidelity}.
  Exposure achieves $r{=}0.997$, Temperature $r{=}0.987$, and Zooming $r{=}0.943$,
  confirming tight coupling between the 1D control input and the rendered effect.
  Bokeh yields $r{=}0.212$; the global blur metric does not capture depth-dependent
  defocus, so the low value reflects proxy mismatch rather than model failure.

  \subsection*{Latent Effect Disentanglement}

  A core motivation of our camera encoder design is that each effect should occupy
  a distinct, non-overlapping region of the latent space.
  We trace where this separation emerges across encoder depth.
  After each forward pass, we capture feature maps at four points:
  (i)~immediately after FiLM modulation at the encoder input,
  and (ii--iv)~after the final attention block of each of the three encoder stages.
  Features are spatially averaged and pooled over time to yield one vector per sample,
  then projected to 2D with t-SNE across ten scenes and all six effects,
  as shown in \cref{fig:latent_disent}.
  Already after FiLM modulation, the six effects form tight, well-separated clusters
  with near-zero within-effect variance across scenes.
  This separation is preserved without collapse through stages~0, 1, and~2,
  showing that the learned per-effect normalization partitions the latent space
  before any temporal modeling occurs.
  The subsequent attention stages refine temporal structure while leaving
  the effect partition intact, validating the disentanglement hypothesis
  underlying our architecture.

\input{content/figures/latent_disentanglement}

  \subsection*{Effect-Stream Dependency} 
  Table~\ref{tab:stream_ablation} reports the effect of zeroing each
  2-D proxy stream independently.
  Removing any individual stream changes PSNR by at most $0.3$\,dB for
  photometric and motion effects, indicating that no single proxy is
  critical when the others remain active.
  The exception is Bokeh, where removing depth reduces PSNR by $0.61$\,dB
  — consistent with its depth-dependent defocus model.
  Zeroing all four streams simultaneously (\textbf{no\_2d}) produces
  similarly small changes, confirming that most 2-D proxies play a
  supporting rather than primary role in effect conditioning.
  Nevertheless, the disentangled multi-stream architecture is a key
  contribution of our design: by dedicating separate latent channels to
  depth, motion, and scene geometry, our framework provides a structured,
  plug-and-play interface for incorporating additional physical scene
  signals, such as surface normals, illumination maps, or material
  properties, without retraining the effect backbone, a capability
  absent from prior camera-control methods.

  \input{content/tables/abla_effect_stream}


\section{Additional Results}



\subsection{Additional Qualitative Results} We present additional qualitative comparisons not presented in the main paper due to lack of space. Specifically, we show the qualitative performance of our model on lens distortion and color temperature vs prior works in \cref{fig:remain_comp}. Further, we directly compare our model with prior works supporting partial intrinsics (only focal length) such as ReCamMaster \cite{bai2025recammaster} in \cref{fig:focal}. We find that our model shows far superior performance in focal length control due to the disentangled training of intrinsics and extrinsics. Further, as shown in the second row is an example with forward camera motion which produces a very similar looking effect as zooming in, where ReCamMaster fails while ours perform better. 

We visualize some of the trajectories extracted by the temporal style extraction module for each effect in \cref{fig:style_extraction_traj}. Since estimating the absolute camera parameter directly from the frame/video is an unfeasible task our model often overshoot or undershoot the camera setting in the starting  frame while still maintaining the change trajectory of the effect over the timesteps. This can also be considered a side effect of our $L_{NCC}$ loss where absolute alignment is not enforced and is left for exploration in future works.

\input{content/figures/recammaster}
\input{content/figures/remain_comp}
\input{content/figures/style_traj}


\input{content/figures/applications}
\subsection{Additional Applications}
We show several examples where our model can be used to invert already existing effects in the input video such as Bokeh deblurring, exposure correction, temperature reversal or zooming out of an already zoomed in video as shown in \cref{fig:applications}.

\subsection{Demo} 

\input{content/figures/demo}
The supplementary archive contains a self-contained HTML viewer \cref{fig:demo}.
To open it, extract the archive and open \texttt{index.html} in any modern web browser (Chrome, Firefox, Edge, Safari).
All video content is loaded locally; no internet connection or installation is required.

If videos do not play from a local file path (some browsers block local media), serve the folder over a local HTTP server:

\begin{verbatim}
cd supp_sigg_sub/
python -m http.server 8080
\end{verbatim}

\noindent Then open \texttt{http://localhost:8080} in your browser.

\subsection*{Directory Structure}

\begin{verbatim}
supp_sigg_sub/
  index.html                        Main viewer
  effect_comparison_videos/         Sec. 1 — main comparison
  comparison_videos3/               Sec. 2 — additional comparisons
  zoom_comparison/                  Sec. 3 — zoom vs. ReCamMaster
  ood_results/                      Sec. 4 — OOD 3-effect results
  supplementary_mixed_style/        Sec. 5 — mixed 2-effect results
  style_transfer_results_supp/      Sec. 6 — camera style transfer
  full_cam_control/                 Sec. 7 — full camera control
  bokeh_match_results_realbokeh/    Sec. 8 — real bokeh matching
  exposure_match_results/           Sec. 9 — real exposure matching
  applications/                     Sec. 10 — applications
\end{verbatim}

\subsection*{Content Overview}

\paragraph{Sec.\ 1 — Main Comparison.}
Side-by-side comparison of our method against VACE~\cite{vace} and CogVideoX~\cite{cogvideox} across all six camera effects (Bokeh, Exposure, Temperature, Zooming, Shutter, Fisheye). Physics-rendered ground truth (GT) is shown for reference.

\paragraph{Sec.\ 2 — Additional Comparisons.}
A second set of source videos with all five methods shown per effect.

\paragraph{Sec.\ 3 — Zoom vs.\ ReCamMaster.}
Our focal-length zoom effect (25$\to$100\,mm) compared against ReCamMaster~\cite{recammaster} dolly-forward, with source and GT shown per video.

\paragraph{Sec.\ 4 — Out-of-Distribution 3-Effect Results.}
Our model applied to three simultaneous effects, including at least two geometric effects not combined during training (e.g., Bokeh + Zooming + Fisheye).

\paragraph{Sec.\ 5 — Mixed 2-Effect Results.}
Fifteen diverse two-effect combinations on RealCam-Vid test videos, with per-sample parameter trajectory plots.

\paragraph{Sec.\ 6 — Camera Style Transfer.}
Camera effect style is extracted from a reference video and transferred onto a new source video, demonstrating disentangled control.

\paragraph{Sec.\ 7 — Full Camera Control.}
Our model conditioned on real extrinsic camera trajectories (pan, tilt, etc.). Each camera type is visualized as a look-direction trajectory on the unit sphere.

\paragraph{Sec.\ 8 — Real Bokeh Matching.}
Aperture and focus sweeps showing our model's output before and after camera-matching fine-tuning on real bokeh video pairs.

\paragraph{Sec.\ 9 — Real Exposure Matching.}
Exposure pairs at 2\,EV and 3\,EV steps, before and after camera-matching fine-tuning.

\paragraph{Sec.\ 10 — Applications.}
Practical application demos including bokeh deblurring, exposure correction, temperature reversal, and zoom-out, each compared against physics-rendered GT.

\section{Limitations} 

\subsection{Failure Modes}
\label{sec:supp_limitations}

\paragraph{Cross-effect leakage in $z_\text{style}$.}
While disentanglement is near-perfect for photometric effects in isolation (InfoNCE $\approx 0.03$, \cref{tab:style_extraction}), we occasionally observe cross-group leakage at inference, most commonly color temperature (ISP group) bleeding into bokeh or fisheye outputs (optical group). \cref{fig:remain_comp} shows an example: a target video conditioned on a fisheye trajectory exhibits a mild concurrent color shift not present in the source. Similarly, \cref{fig:applications} (right, bottom) shows an example of reversing zoom in the source video leads to \textit{leaky} adjustment of color temperature. This indicates the per-group FiLM cascades are not perfectly isolated in practice; we suspect residual coupling through the shared spatial proxy features. Adding an explicit cross-group orthogonality loss is a natural next step.

\paragraph{Output resolution and backbone scale.}
All results use Wan-2.1 at 1.3B and 480$\times$832, the smallest configuration we could run on our hardware budget (single A6000, 96GB). Fine high-frequency texture and small-object fidelity therefore lag larger 5B+ backbones at 720p/1080p, most visibly on effects relying on sub-pixel structure (low-intensity lens distortion, narrow depth-of-field on small subjects). Our contributions are backbone-agnostic and should transfer to larger VDM variants without redesign.

\paragraph{Reliance on deterministic spatial proxies.}
Intrinsic conditioning depends on off-the-shelf depth, flow, and perspective-field estimators; failures propagate into generation. We observe degradation in (1) heavy global motion blur (unreliable flow), (2) transparent and refractive surfaces (incorrect depth), and (3) extreme source distortions violating pinhole assumptions (\cref{fig:limitations}). Uncertainty-aware proxies or proxy-noise-robust conditioning are natural future directions.

\paragraph{Synthetic-to-real gap.}
Stages 1--2 train on synthetic camera-paired video; only Stage 3 grounds to real EXIF captures, and only for bokeh, exposure, and zoom. Generalization to cameras whose sensor characteristics are not represented in our synthetic pipeline (e.g., medium-format, anamorphic) is empirically reasonable but not quantified.

% \section{Code}

% \section{How to use this template}

% This \LaTeX{} template was developed to (1) streamline collaborative manuscript editing and (2) automate many processes that manu\-scripts undergo throughout the publication process of academic papers.
% Many ideas, features, and aspects in this template were adapted from my previous collaborators and mentors such as Qi Sun, Li-Yi Wei and Jane Hoffswell.

% \subsection{Usage}

% The \LaTeX{} compilation is managed by a \texttt{Makefile}.
% The \texttt{Makefile} features multiple build targets meant for various versions of the document, such as \texttt{internal} for sharing between collaborators, and \texttt{submission} for anonymous submissions.
% These targets are built by running \texttt{make <target\_name>} (\eg \texttt{make internal}).
% See \Cref{sec:howto:build-pipeline} for details on the various build targets.

% \paragraph{Pre-requisites}
% The \texttt{Makefile} assumes the usage of \texttt{pdflatex}, so please make sure to install the \texttt{texlive}, \texttt{texlive-latex-extra}, \texttt{texlive-fonts-recommended}, \texttt{texlive-science}, and \texttt{texlive-x\hfill\break string} packages.
% Additionally, \texttt{ghostscript} is used for post-com\-pilation PDF document processing such as to separate the document into separate files for the manuscript and supplementary materials.
% See more details on this in \Cref{sec:howto:build-pipeline}.

% \subsection{\LaTeX{} macros for collaborative editing}
% \label{sec:howto:macros}

% This template features a number of very convenient macros designed to make collaborative writing much easier and more streamlined.
% All of these macro definitions can be found in \texttt{conf/macros.tex} and edited as necessary.
% Below, we outline what the features are and how to use them.

% \paragraph{Tracking Progress: Status Badges and To-do Items}
% When collaborating on a large document, it's often helpful to keep track of what sections have been reviewed, what sections are complete \etc
% This template enables status tracking of paper sections via \emph{Status Badges} as well as \emph{To-do Item} annotations which can be viewed in summary at the top of the document.

% \emph{Status Badges} indicate what state a particular section of the manuscript is in and allows collaborators to claim, and release sections as necessary.
% To add a badge to a section, simply add the corresponding badge command at the end of the section title
% (\eg \texttt{\textbackslash section\{Section Title \textbackslash incomplete\}}).
% This badge will not only annotate the section title with its corresponding status, but also include the annotation to a summary \Quote{table-of-contents} which appears at the top of the document when rendered in the \texttt{internal} version.
% For the full list of possible status badges, see \Cref{tab:howto:status-badges}.
% %
% \begin{table}[ht]
%     \caption{Status badges}
%     \label{tab:howto:status-badges}
%     \begin{tabular}{ll}
%         \toprule
%         Command & Created Badge\\
%         \midrule
%         \texttt{\textbackslash incomplete} & \incomplete\\
%         \texttt{\textbackslash underRevision} & \underRevision\\
%         \texttt{\textbackslash feedbackNeeded} & \feedbackNeeded\\
%         \texttt{\textbackslash feedbackGiven} & \feedbackGiven\\
%         \texttt{\textbackslash complete} & \complete\\
%         \texttt{\textbackslash locked} & \locked\\
%         \bottomrule
%     \end{tabular}
% \end{table}

% \emph{To-do Items} are also a helpful tool for annotating important to-do items that need to be tracked.
% Including an actionable in the source document as \texttt{\textbackslash todo\{revise this sentence\}} will render the to-do item within the manuscript in a highlighted red color, and also include a copy of this to-do item in the \Quote{table-of-contents} at the top of the document just like the \emph{Status Badges}.

% The combination of these two macros can help collaborators keep track of everything that still needs to be done for a paper submission prior to deadlines.

% \paragraph{Exchanging feedback via in-document comments}
% In addition to important to-do items, sometimes it is helpful to simply have asynchronous discussions that aren't necessarily mission critical within the document draft itself.
% To facilitate this workflow, the template also supports macros for in-document comments by multiple collaborators, each highlighted in a different color.
% \monde{For example, I might have some thoughts on the organization of this section.}
% \qisun{And I might respond to Monde's concerns in response.}

% The current template has pre-defined macros for four collaborators: \texttt{monde}, \texttt{qi}, \texttt{anjul}, and \texttt{rachel}.
% To use the macro call the macro as \texttt{\textbackslash monde\{comment contents\}} for a simple comment.
% \monde[To annotate existing text to reference by the comment,]{like this,}\break
% put the existing text into square brackets.
% For example, \texttt{\textbackslash monde[anno\hfill\break tated text]\{comment contents\}}.
% There is also a generic \texttt{guest} command to allow a guest to input their name into their comment without having to define a new macro.
% To use this version, call the macro as \texttt{\textbackslash guest\{name\}\{comment contents\}} for a simple comment and \texttt{\textbackslash guest[annotated text]\{name\}\{comment contents\}} for annotated comments.

% \paragraph{Revision annotation}
% During the revision stage of a document for publication, reviewers often ask for specific edits to the manuscript.
% To enable an easy back and forth between the reviewer and the authors, highlighting all the changed text can be very helpful.
% To this end, this template features a \texttt{\textbackslash revise\{text to remove\}\{text to add\}} macro which annotates both removed and added text.
% By inputting the to-be-removed text in the first argument, and the to-be-added text in the second argument, the annotation \revise{won't}{will} look like this.
% By default, the removed text will only be shown in the \texttt{internal} version of the document, while the \texttt{revision} version of the document only shows the added text.
% But you can edit this behavior in the \texttt{conf/macros.tex} file.
% The automated build pipeline (\cf \Cref{sec:howto:build-pipeline}) allows seamless changes between the different versions of how a revised text should be rendered.

% \subsection{File Organization}

% This template is organized into a granular structure and logical separation of various types of source files that make up a \LaTeX{} document.
% \Cref{tab:howto:path-description} explains what types of files are at the various paths.
% %
% \begin{table}[ht]
%     \caption{File paths and their functions}
%     \label{tab:howto:path-description}
%     \begin{tabular}{ll}
%         \toprule
%         Path & Function\\
%         \midrule
%         \texttt{sections} & numbered section \LaTeX{} source files\\
%         \texttt{sections/abstract.tex} & document abstract\\
%         \texttt{sections/acks.tex} & acknowledgements section\\
%         \texttt{sections/document.tex} & manuscript sections entry point\\
%         \texttt{sections/readme.tex} & how to use this template\\
%         \texttt{sections/supp.tex} & supp. material entry point\\
%         \texttt{tables} & table \LaTeX{} source files\\
%         \texttt{figures} & figure \LaTeX{} source files\\
%         \texttt{assets} & illustrations and plots\\
%         \texttt{conf} & \LaTeX{} configurations\\
%         \texttt{metadata} & metadata of the document\\
%         \texttt{targets} & \LaTeX{} compilation entry points\\
%         \texttt{paper.tex} & combination of source files\\
%         \texttt{paper.bib} & bibliography\\
%         \texttt{Makefile} & build pipeline definitions\\
%         \texttt{build} & build outputs\\
%         \bottomrule
%     \end{tabular}
% \end{table}

% \paragraph{Sections}
% All numbered sections are combined in \texttt{sections/docu\hfill\break ment.tex}, which in turn are inputted in the compilation process in \texttt{paper.tex}.
% Each numbered section name is prepended by its number for visual clarity, and each section is given its \LaTeX{} label in the form \texttt{\textbackslash label\{sec:<section\_name>\}}.
% Further subsection labels are nested as \texttt{sec:<section\_name>:<subsection\_name>}.

% \paragraph{Tables and Figures}
% All table and figure source files are separated from \emph{Section} source files to enable easy edits to where a figure should be added in the source.
% Each figure is given its \LaTeX{} label in the form \texttt{\textbackslash label\{tab:<table\_name>\}} or \texttt{\textbackslash label\{fig:figure\_name\}}

% \paragraph{Packages, Aliases, and Macros}
% \LaTeX{} package imports are consolidated in \texttt{conf/packages.tex}.
% To avoid complications when some packages need to be deprecated in the future, it's advised that the specific usage of each package is documented as a comment.
% For example, we use the \texttt{soul} package to enable underlining and strike-through functionality for annotating collaborator comments, and text revisions.
% If in the future, either this feature of the template is changed or removed, removing this package dependency will be much easier to identify and execute.

% All symbol aliases used during writing are consolidated within \texttt{conf/symbols.tex}, while more complex macros are in \texttt{conf/macro\hfill\break s.tex}.
% More details on what kind of macros are used in this template are in \Cref{sec:howto:macros}.

% \paragraph{Paper metadata}
% All source files pertaining to paper metadata, such as the title, authors, journal number, publication year \etc are included in \texttt{metadata/} and are self-explanatory.
% These metadata fields are inserted into the compilation in \texttt{paper.tex}.
% If you're changing the document class, include any document class related metadata fields in the \texttt{metadata/} directory, and change the organization of source files within \texttt{paper.tex}.

% \paragraph{Build targets}
% All build targets have their associated \LaTeX{} entry point inside \texttt{targets/} as well as a  \texttt{Makefile} target.
% See more details about the build pipeline in \Cref{sec:howto:build-pipeline}.

% \subsection{Build Pipeline}
% \label{sec:howto:build-pipeline}

% The build process of the manuscript is fully automated via a \texttt{Makefile} and allows the user to seamlessly produce different versions of the manuscript and supplementary materials documents.
% \ie the document can be produced at various stages of \Quote{readiness for publication}, with each different stage revealing or hiding various comments and annotations.
% The supported document stages are described in \Cref{tab:howto:doc-stages}.
% %
% \begin{table}[ht]
%     \caption{Document stages and their usage and features.}
%     \label{tab:howto:doc-stages}
%     \begin{tabular}{ll}
%         \toprule
%         Build target & Usage and features\\
%         \midrule
%         \texttt{internal} & internal collaborative use with comments shown\\
%         \texttt{submission} & anonymous submission with no annotations\\
%         \texttt{revision} & annotated anonymous revision for reviewers\\
%         \texttt{camready} & final camera-ready with author names shown\\
%         \texttt{camauthor} & author-version for sharing post-publication\\
%         \bottomrule
%     \end{tabular}
% \end{table}

% You may add additional document stages by
% %
% \begin{itemize}
%     \item adding a new \LaTeX compilation entry file inside \texttt{targets/},
%     \item updating the \texttt{Makefile} targets, and
%     \item adding your custom logic for what annotations to enable in \texttt{conf/macros.tex}.
% \end{itemize}

% \paragraph{Automated manuscript and supp. material separation}
% Often a paper publication requires an associated supplementary materials section for any exposition that does not central to the publication and are omitted from the main manuscript.
% In order to take advantage of \LaTeX{} cross-referencing features, such as \texttt{\textbackslash Cref}, it's best to compile all the source files in one batch and generate a single PDF output.
% However, doing so requires post-processing on the outputted file to separate them into multiple PDFs via an external application such as Adobe Acrobat \etc
% Additionally, many paper templates also print the number of pages of the document which include the supplementary material pages if this method is used to generate two separate files for the main manuscript and the supplementary material.

% This template takes care of these manual steps and also solves the page count issue and keeps all the complexity of the compilation and post-processing logic tucked away in the \texttt{Makefile}.
% In order to take advantage of this feature, make sure to use the Makefile to compile your document and have its dependent \texttt{ghostscript} package installed on your machine.

% \subsection{Future Features}
% \label{sec:howto:future-features}

% I'm constantly updating this template to help make the paper authoring and collaboration process more streamlined.
% Below is a short list of features that I'm looking to add in the future:
% %
% \begin{itemize}
%     \item add easy to use \LaTeX{} linting and formatting scripts;
%     \item add helper scripts which \Quote{commit/revert} the revisions by stripping the \LaTeX{} tags and incorporating the existing revisions into the native text;
%     \item add a \texttt{Makefile} target for preparing the publication for Arxiv upload;
%     \item streamline the process of swapping out different style files;
%     \item split the package dependencies so that unnecessary development / internal dependencies are omitted;
%     \item add a script which \Quote{dumbs down} the \LaTeX{} source files into a single source file to satisfy strict publisher requirements.
% \end{itemize}
